# Supplementary material for: A Unified Model for Multi-class Anomaly Detection
Source: arXiv:2206.03687 source file (2022-10-25)
Supplement: Supplementary file 1 [file 0.1.overview.tex]

\section{Overview}\label{appendix:sec:overview}

We organize the supplementary material as follows. 
\cref{sec:setting} discusses the setting of our proposed unified case. 
\cref{appendix:sec:architecture} describes the detailed architecture of the three baseline reconstruction networks (MLP, CNN, and transformer), our \method, and other assistant modules, followed by the training configurations.
\cref{appendix:sec:ablation} conducts comprehensive ablation studies on the components of our approach.
\cref{appendix:sec:results} presents more visualization results of the reconstructed features and qualitative results for anomaly localization on MVTec-AD~\cite{mvtec} under the unified case.
