# Supplementary material for: A Unified Model for Multi-class Anomaly Detection
Source: arXiv:2206.03687 source file (2022-10-25)
Supplement: Supplementary file 2 [file 5.ref.tex]

{\small
\bibliographystyle{abbrvnat}
\bibliography{ref}
}
